# Supplementary material for: Partial Selfish Mining for More Profits
Source: arXiv:2207.13478 source file (2024-04-06)
Supplement: Supplementary file 1 [file DynamicStrategy.tex]

\section{Appendix}%本节存疑
~\label{sec: StrategySelect}
%\subsection{Proof of Theorem 4.1}
%As discussed in section ~\ref{sec:simulation}, there is no dominant one-size-fits-all strategy for all parameters. Attackers must carefully choose the mining strategy based on its mining power and the network condition. When the attacker's mining power is relatively small, honest mining is the best choice. But if the attacker's mining power is large enough, selfish mining can get more revenue. It is necessary to determine the mining strategy based on the information attackers can get. In this section, we model the combination of different mining strategies as a mining strategy selection process. 

%This section further analyzed the three mining strategies and proposed an optimal mining strategy selection mechanism that enables the attacker always to select the most profitable mining strategy.

%\subsection{Overview}

%Instead of choosing a specific mining strategy, in this section, we assume that the attacker can choose a combination of different mining strategies, and adjust the execution time to see if attackers could get a higher profit. To do this, we proposed a mining strategy selection mechanism.

%\subsubsection{Strategy Description}

\begin{figure}[htbp]
	\centerline{\includegraphics[width=\columnwidth]{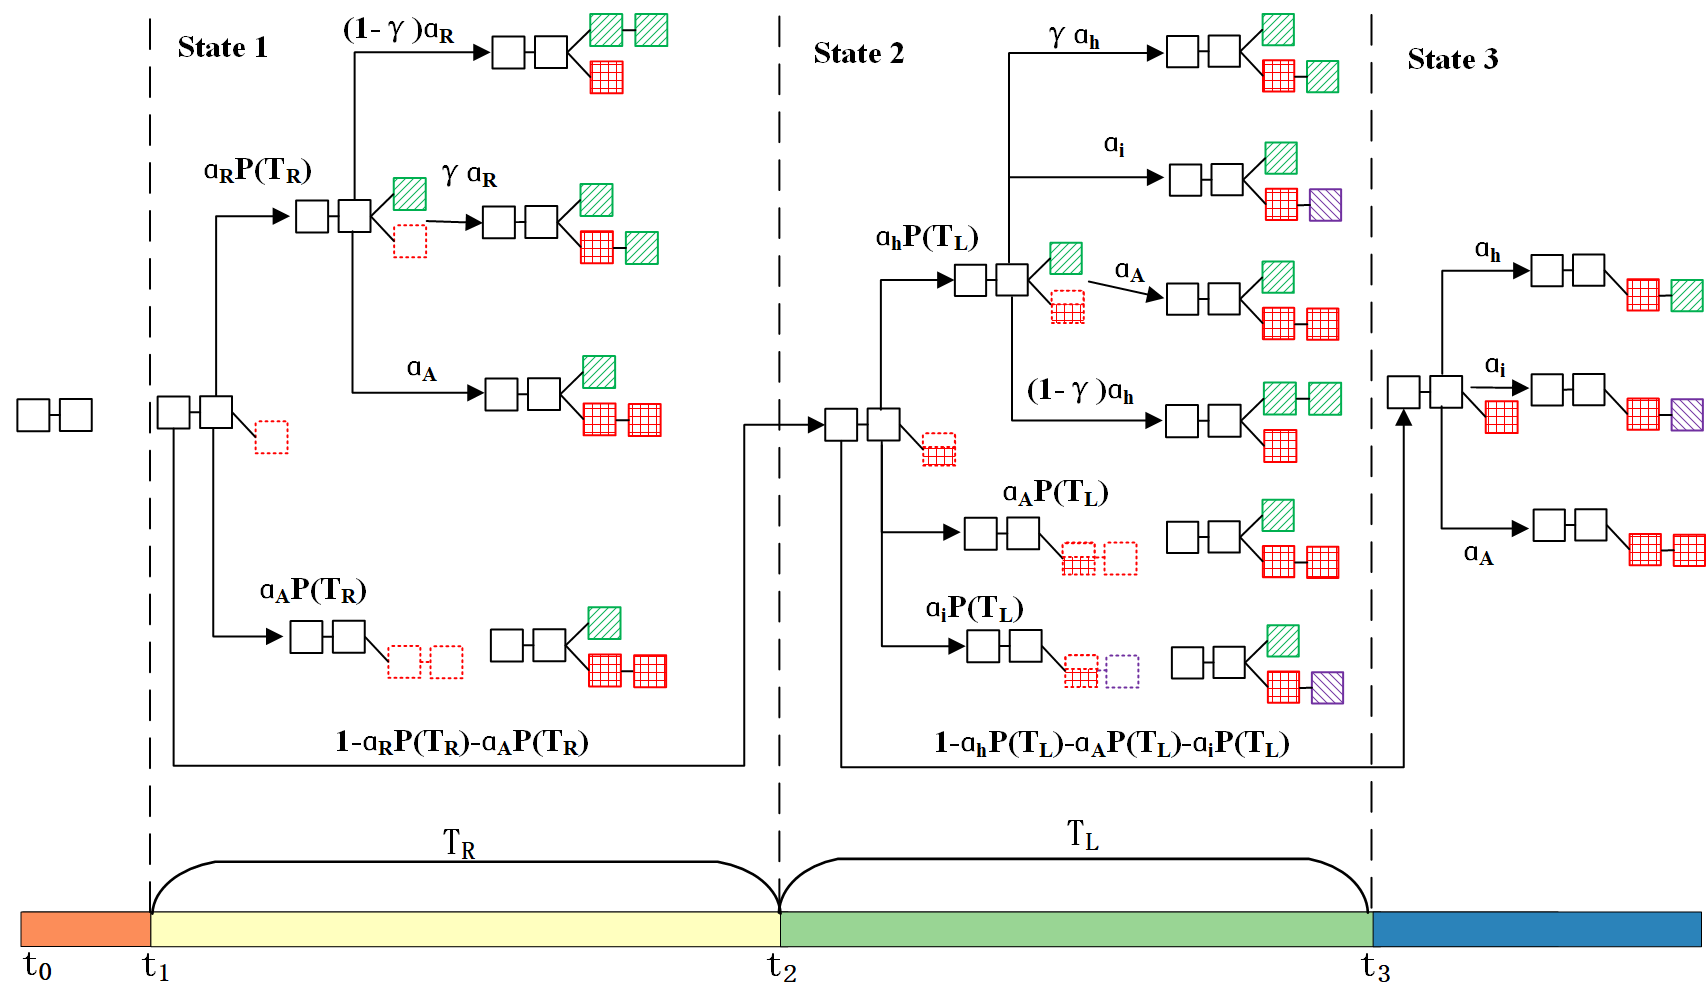}}
	\caption{Workflow of the mining strategy selection mechanism}
	\label{fig:Overview}
\end{figure}
The workflow of the general partial block sharing process is shown in Figure \ref{fig:Overview}. 

\nop{
The workflow of the general partial block sharing process is shown in figure ~\ref{fig:Overview}. When the attacker finds a block, it will keep the block private for a certain time $T_R$ instead of publishing the new block. During this time period, the attacker does the selfish mining. If the attacker finds a new block during $T_R$, it continues to follow the original selfish mining and will not proceed to the next state. When other miners find a block in the public chain, if the attacker has a comfortable lead of two-block, then it will release its private branch and get the revenue of all its two blocks. If the attacker's lead is more than two blocks, the attacker will release one block at a time until the lead is reduced to 2. Since the attackers' mining power is less than two, the system will eventually return to the single branch state. 

If other miners find the new block during the period $T_R$, the attacker releases its private branch and starts a 0-lead racing. In this scenario, the attacker will mine on the previously private branch, and the other miners will choose to mine on either branch. As we have defined earlier, $\gamma$ miners will mine on the private branch, and $1-\gamma$ miners will mine on the public branch.

If neither the attacker nor other miners find the new block during $T_R$, then the system will proceed into the next state. 

In State 2, the attacker will continue to mine on the private branch for $T_L$. In the meantime, it will release the partial Attackers will release a smart contract that allows miners to get block hash as well as the block body privately so that miners can mine on the private chain. Then there are four possible cases in this scenario: the attacker finds the new block in its private chain, other miners find a new block on the public branch, other miners find a new block in the private branch, or none of the miners find a new block. These scenarios have been discussed in section~\ref{sec:ATKOverviewAndStr}. If none of the miners find the new block, then the system will proceed into State 3.

In state 3, the attacker will release the block, and the system backs to the single branch state.
}

%\subsubsection{Block Generation Time}

%\subsection{Revenue Evaluation}

%TODO:定义好ah,ar和ai%

%As is shown in figure~\ref{fig:Overview}, our strategy allows the attacker to gain a revenue larger than its ratio of mining power. Besides, it can also attract some miners to join its mining process and gain more rewards together with the miner. 

In the first state of the partial block sharing process, when the attacker first finds a new block, it can choose to do the selfish mining for time period $T_R$ or release the partial block immediately ($T_R=0$). 

Then three possible cases may happen:

Case1.1: the honest miner finds the block. Then the attacker will release the block immediately and start a 0-lead racing with other miners. Then there will be three sub-cases:

Case1.1.1: The honest miner find the new block after the honest miner's branch. In this case, the honest miner will get two-block rewards. The possibility is $(1-\gamma)\alpha_R$. The revenue of each participant can be represented as:
\begin{equation}
		  R_{1.1.1}^A=0, \     \ R_{1.1.1}^R=2\alpha_RP(T_R)\times(1-\gamma) \alpha_R . 
\end{equation}
Case 1.1.2: The honest miner finds the new block after the attacker's branch. In this case, the attacker will get 1 block reward, and the honest miner will get 1 block reward. The possibility is $\gamma \alpha_R$. The revenue of each participant can be represented as:
\begin{equation}
		  R_{1.1.2}^A= R_{1.1.2}^R=  \alpha_R P(T_R)\times \gamma \alpha_R 
\end{equation}

Case 1.1.3: The attacker finds the new block. In this case, the attacker will get 2 block rewards. The possibility is $\alpha_A$. The revenue of each participant can be represented as:
\begin{equation}
		 R_{1.1.3}^A=2 \alpha_R  P(T_R)\times \alpha_A,\     \  R_{1.1.3}^R=0. 
\end{equation}
%\begin{subequations}
%	\begin{align}
%		 &R_{1.1.3}^A=2\tmies \alpha_R \times P(T_R)\times\alpha_A.   \\ 
%		 &R_{1.1.3}^R=0. 
%	\end{align}
%\end{subequations}

Case1.2: the adversary finds the block. In this case, when other miners find a new block, the adversary will release the two-block immediately. The possibility of entering this scenario is the possibility of the attacker finding a new block within time $T_R$, which can be written as $\alpha_A \times P(T_R)$. In this scenario, only the attacker can get 2 blocks of revenue. The revenue of each participant can be represented as:

\begin{equation}
		 R_{1.2}^A=2 \alpha_A P(T_R),\     \ R_{1.2}^R=0. 
\end{equation}

Case1.3: Neither the adversary nor the miners find the new block. In this case, the strategy will proceed to state 2. 

Overall, the attacker's revenue in state 1 can be represented as:
\begin{equation}
\begin{aligned}
    R_1^A&= R_{1.1.2}^A+R_{1.1.3}^A+R_{1.2}^A\\
   & =\alpha_R P(T_R)(\gamma\alpha_R+2\alpha_A)+2 \alpha_A  P(T_R),
    \end{aligned}
\end{equation}

the other miners' revenue is:

\begin{equation}
\begin{aligned}
    R_1^R&= R_{1.1.1}^R+R_{1.1.2}^R\\
    &=\alpha_R P(T_R)\times (\gamma\alpha_R+2(1-\gamma)\alpha_R),
    \end{aligned}
\end{equation}
and the possibility of entering the state 2 is:
\begin{equation}
    P_2= 1-\alpha_R P(T_R)-\alpha_A  P(T_R).
\end{equation}

In State 2, the attacker will share the partial block with rational miners. In this state, four possible cases may happen.

Case 2.1: Honest miners find the new block. Then four possible sub-cases may happen:

Case 2.1.1: Honest miners find the new block after the honest miner's branch. In this case, the honest miner will get two block rewards. The possibility is $(1-\gamma)\alpha_h$. The revenue of each participants can be represented as:
\begin{equation}
	\begin{aligned}
		  &R_{2.1.1}^A=R_{2.1.1}^i=0  \\ 
		 &R_{2.1.1}^h=2 \alpha_h  P(T_L)\times(1-\gamma)\alpha_h. 
	\end{aligned}
\end{equation}

Case 2.1.2: Honest miners find the new block after the attacker's branch. In this case, the attacker will get 1 block reward and the honest miner will get 1 block reward. The possibility is $\gamma \alpha_h$. The revenue of each participants can be represented as:
\begin{equation}
	\begin{aligned}
		  &R_{2.1.2}^A=\alpha_h  P(T_L)\times\gamma\alpha_h , R_{2.1.2}^i=0  \\ 
		 &R_{2.1.2}^h=2 \alpha_h  P(T_L)\times(1-\gamma)\alpha_h. 
	\end{aligned}
\end{equation}

Case 2.1.3: The attacker finds the new block. In this case, the attacker will get 2 block rewards. The possibility is $\alpha_a$. The revenue of each participants can be represented as:

\begin{equation}
	\begin{aligned}
		  &R_{2.1.3}^A=2\alpha_h P(T_L)\times(1-\gamma)\alpha_h  \\ 
		   &R_{2.1.3}^i=R_{2.1.3}^h=0.
	\end{aligned}
\end{equation}

Case 2.1.4: Greedy miners find the new block. In this case, the attacker will get 1 block reward and the greedy miner will get 1 block reward. The possibility is $\alpha_i$. The revenue of each participants can be represented as:
\begin{equation}
	\begin{aligned}
		 &R_{2.1.4}^A= R_{2.1.4}^i=\alpha_h  P(T_L)\times\alpha_i,   \\ 
		 &R_{2.1.4}^h=0.
	\end{aligned}
\end{equation}

Case 2.2:  The attacker finds the block. In this case, the attacker will release the two block immediately. In this case, the adversary will get 2 block rewards. The revenue of each participants can be represented as:
\begin{equation}
	\begin{aligned}
		 &R_{2.2}^A= 2\alpha_A P(T_L)  \\ 
		 &R_{2.2}^i=R_{2.2}^h=0.
	\end{aligned}
\end{equation}

Case 2.3:  Greedy miners find the block. In this case, the attacker will release the two blocks immediately. In this case, the adversary will get 1 block reward, and the greedy miner will get 1 block reward. The revenue of each participant can be represented as:
\begin{equation}
		 R_{2.3}^A=  R_{2.3}^i=\alpha_i P(T_L),   \     \ R_{2.3}^h=0.
\end{equation}

Case 2.4: None of the miners find the new block. In this case, the attacker will release the private branch, and then the blockchain goes back to the single branch state.

Overall, the attacker's revenue in state 2 can be represented as:
\begin{equation}
\begin{aligned}
    R_2^A&= R_{2.1.2}^A+R_{2.1.3}^A+R_{2.1.4}^A+R_{2.2}^A+R_{2.3}^A\\
    &=\alpha_h  P(T_L)\times\gamma\alpha_h+2 \alpha_h  P(T_L)\times(1-\gamma)\alpha_h+\\
    &\alpha_h  P(T_L)\times\alpha_i+2 \alpha_A  P(T_L)+\alpha_i  P(T_L),
    \end{aligned}
\end{equation}

the greedy miners choosing to participate in the private branch's revenue are:

\begin{equation}
\begin{aligned}
    R_2^i&= R_{2.1.4}^i+R_{2.3}^i=\alpha_h  P(T_L)\times\alpha_i+\alpha_i  P(T_L),
    \end{aligned}
\end{equation}

the honest miners' revenue is:

\begin{equation}
\begin{aligned}
    R_2^h&= R_{2.1.1}^h+R_{2.1.2}^h\\
    &=2\alpha_h  P(T_L)\times(1-\gamma)\alpha_h+2\alpha_h  P(T_L)\times(1-\gamma)\alpha_h,
    \end{aligned}
\end{equation}

and the possibility of going back to the single branch state is:
\begin{equation}
    P_{exit}= 1- P(T_L).
\end{equation}

We can derive the attacker's revenue as:

\begin{equation}
\begin{aligned}
&R_A^S=R_1^A+R_2^A\\
&=2 \alpha_A  P(T_R )+\gamma  \alpha_R ^2 P(T_R )+2 \alpha_A \alpha_R  P(T_R )+\\
&(1- P(T_R )) (2 \alpha_A  P(T_L )+\alpha_i  P(T_L )+\\
    &2 \alpha_A\alpha_h  P(T_L )+\alpha_i \alpha_h  P(T_L )+\gamma  \alpha_h^2 P(T_L )+\\
    &((1- P(T_L)) (2\alpha_A+\alpha_i+\alpha_h))).
\end{aligned}
\end{equation}

If the attacker chooses to follow the honest mining strategy, then it will surely get 1 block revenue, and the possibility of getting the second revenue is $\alpha_A$. So, if the attacker chooses honest mining, the revenue is:
\begin{equation}
    R_A^H =1+\alpha_A
\end{equation}.
%\subsection{For the attacker, how to choose $T_L$ and $T_R$ can get the most revenue?}

%We assume that the attacker may choose three strategies: 1. selfish Mining, 2. partial block sharing, and 3. honest mining. Here, we are interested in what strategies can maximize the attacker's revenue.

%To answer the problem, first, we need to figure out how to choose $T_L$, and $T_R$ can maximize the reward of attacker. To be specific, it needs to solve the following problem:

\textbf{(Problem)} Attacker revenue maximization: With given $\alpha_A$, $\alpha_i$ and $\gamma$, attacker revenue maximization is to maximize the attacker's revenue $R_A^S$ by choosing appropriate $T_L$ and $T_R$. This problem can be formally formulated as: 
\begin{subequations}\label{eq:atk1}
	\begin{align}
		  & \underset{T_R,T_L}{\text{Maximize}} &&  R_A^S,  \\ 
		 & \text{s.t.} && \alpha_A+\alpha_i+\alpha_h=1,\\ & &&
		 \alpha_A+\alpha_R=1,\\ & && 
		\alpha_A<0.5,\\ & && 0<\gamma<1.
	\end{align}
\end{subequations}
To solve the problem, first taking the partial derivatives with respect to $T_L$ and $T_R$ respectively, let $dT_L$ be the partial derivative of $R_A^S$ with respect to $T_L$, and $dT_R$ be the partial derivative of $R_A^S$ with respect to $T_R$, we can get:
\begin{equation}
\begin{aligned}
    dT_L=&(((-\alpha_i^2)+(2-2\alpha_A)\alpha_i-\alpha_A^2+2\alpha_A-1)\gamma+\\
    &\alpha_i^2+(3\alpha_A-2)\alpha_i+2\alpha_A^2-3\alpha_A+1)P(T_R)+\\
    &(\alpha_i^2+(2\alpha_A-2)\alpha_i+\alpha_A^2-2\alpha_A+1)\gamma-\\
    &\alpha_i^2+(2-3\alpha_A)\alpha_i-2\alpha_A^2+3\alpha_A-1,
    \end{aligned}
\end{equation}
\begin{equation}
\begin{aligned}
    dT_R=&(((-\alpha_i^2)+(2-2\alpha_A)\alpha_i-\alpha_A^2+2\alpha_A-1)\gamma+\\
    &\alpha_i^2+(3\alpha_A-2)\alpha_i+2\alpha_A^2-3\alpha_A+1)P(T_L)+\\
    &(\alpha_A^2-2\alpha_A+1)\gamma-2\alpha_A^2+3\alpha_A-1
    \end{aligned}
\end{equation}

Let $dT_L=0$, then we can get $P(T_R)=1$. That means $R_A^S$ is monotonic when $P(T_R)\in [0,1)$. Take any $T_R\geq 0$, if $dT_L>0$, means  $R_A^S$ increases monotonically as $T_L$ increases. PSM is more profitable than honest mining, but it still need to calculate the value of $dT_R$ to see if the PSM is more profitable than BSM. If $dT_L<0$, means attacker should not spend any time on PSM, $T_L=0$.

With $T_L=0$, we can get the value of $dT_R$. If $dT_R>0$ means selfish mining is the most profitable strategy. If $dT_R<0$ and $dT_L>0$ means the PSM is the most profitable strategy.  Otherwise, the attacker should choose honest mining because neither PSM nor selfish mining can get more rewards than honest mining for the attacker.
